# Supplementary material for: Measuring Absolute Velocities from Non-Equilibrium Oscillations via Single-Detector 3D Dynamic Light Scattering
Source: arXiv:2404.02217 source file (2024-10-07)
Supplement: Supplementary file 1 [file SM_PRL_Oscillation.pdf]

# **Measuring Absolute Velocities using Non-Equilibrium Oscillations via Single-Detector 3D Dynamic Light Scattering**

José López-Molina,<sup>1</sup> Arturo Moncho-Jordá,<sup>1,2,\*</sup> and María Tirado-Miranda<sup>1,†</sup>

<sup>1</sup>*Department of Applied Physics, Universidad de Granada,  
Campus Fuentenueva S/N, 18071 Granada, Spain.*

<sup>2</sup>*Institute Carlos I for Theoretical and Computational Physics,  
Universidad de Granada, Campus Fuentenueva S/N, 18071 Granada, Spain.*

(Dated: October 7, 2024)

## SUPPLEMENTAL MATERIAL

### A. Two-Laser Single-Detector Correlation Function in Dynamic Light Scattering with One Drift Velocity

Dynamic Light Scattering (DLS) experiments invariably encompass three integral elements positioned within a plane: a light source, a colloidal system inducing light scattering, and a detector situated at an angle  $\theta$  relative to the incident beam. The detector quantifies the intensity of the system-scattered light as a function of time, denoted as  $I(\mathbf{q}, t)$ . To elucidate pertinent information from this signal, the intensity autocorrelation function  $g^{(2)}(\mathbf{q}, \tau)$  is employed [1, 2]:

$$g^{(2)}(\mathbf{q}, \tau) = \frac{\langle I(\mathbf{q}, 0)I(\mathbf{q}, \tau) \rangle}{\langle I(\mathbf{q}, 0) \rangle^2} \quad (\text{S1})$$

Here,  $\tau$  represents the correlation time, and  $\mathbf{q}$  signifies the scattering vector, defined as  $\mathbf{q} = \mathbf{k}_i - \mathbf{k}_f$ , with  $\mathbf{k}_i$  and  $\mathbf{k}_f$  being the wave vectors of the incident and scattered waves, respectively. The angular brackets denote ensemble averaging.

This research centers on colloidal systems with monodisperse, non-interacting particles, thereby satisfying the Siegert relation which connects the intensity correlation function  $g^{(2)}(\mathbf{q}, \tau)$  with the electric field correlation function  $g^{(1)}(\mathbf{q}, \tau)$  [3–6]:

$$g^{(2)}(\mathbf{q}, \tau) = 1 + |g^{(1)}(\mathbf{q}, \tau)|^2 \quad (\text{S2})$$

This relationship facilitates the model development by considering the electric field. The correlation function of the electric field is expressed as:

$$g^{(1)}(\mathbf{q}, \tau) = \frac{G^{(1)}(\mathbf{q}, \tau)}{G^{(1)}(\mathbf{q}, 0)} \quad (\text{S3})$$

where  $G^{(1)}(\mathbf{q}, \tau)$  is the non-normalized correlation function of the scattered electric field  $E_s(\mathbf{q}, t)$

$$G^{(1)}(\mathbf{q}, \tau) = \langle E_s(\mathbf{q}, 0)E_s^*(\mathbf{q}, \tau) \rangle \quad (\text{S4})$$

We start considering a flat monochromatic electromagnetic wave, described by the electric field  $\mathbf{E}_i(\mathbf{r}, t)$  at a point  $\mathbf{r}$  and time  $t$ . This wave has a wavelength  $\lambda_i$ , frequency  $\omega_i$ , polarization  $\mathbf{n}_i$

---

\* moncho@ugr.es.

† mtirado@ugr.es.

perpendicular to the plane, and amplitude  $E_0$ . The wave also has a wave vector  $\mathbf{k}_i$  pointing to the direction of propagation of the incident wave, defined as:

$$\mathbf{k}_i = \left( \frac{\omega_i}{c} \right) \hat{\mathbf{k}}_i$$

where  $c$  is the speed of light. The electric field of the incident wave is given by:

$$\mathbf{E}_i(\mathbf{r}, t) = \mathbf{n}_i E_0 e^{i(\mathbf{k}_i \cdot \mathbf{r} - \omega_i t)} \quad (\text{S5})$$

This incident wave arrives to the dispersion of colloidal particles, each of which scatters without changing the frequency of the incident wave. A detector is placed at an angle  $\theta$  to the incident direction as shown in Fig. S1. It collects the scattered radiation, which has the same polarization that the incident beam,  $\mathbf{n}_f = \mathbf{n}_i$ . We consider the scattering induced by a single colloidal particle  $\alpha$  located at position  $\mathbf{r}_\alpha(t)$  that arrives to the light detector placed at position  $\mathbf{R}$ , both with respect to the light source. The wave travels from the source to the particle position  $\mathbf{r}_\alpha(t)$  with a wave vector  $\mathbf{k}_i$ , is scattered by the particle, and then travels a distance  $\mathbf{R} - \mathbf{r}_\alpha(t)$  to reach the detector with a wave vector  $\mathbf{k}_f$ . We denote by  $\theta$  the angle formed between the incident and the scattered light.

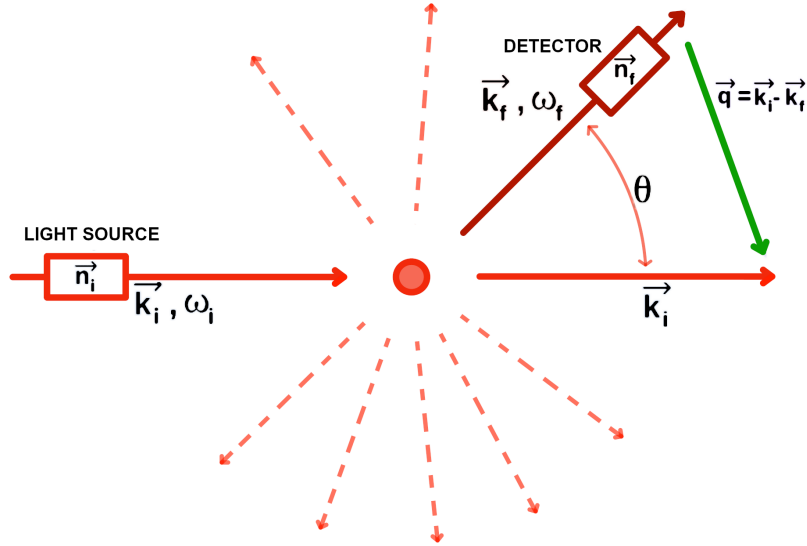

FIG. S1. Electromagnetic wave with wave vector  $\mathbf{k}_i$  strikes a particle and is scattered. At an angle  $\theta$ , the scattered wave with wave vector  $\mathbf{k}_f$  and polarization  $\mathbf{n}_f$  reaches the detector.

The electric field from laser  $l$  scattered by particle  $\alpha$  and arriving at the detector can be expressed as:

$$\mathbf{E}_{l,\alpha}(\mathbf{q}, t) = \mathbf{n}_i E_{l,\alpha}(\mathbf{q}) e^{i[\mathbf{k}_i \cdot \mathbf{r}_\alpha(t) + \mathbf{k}_f \cdot (\mathbf{R} - \mathbf{r}_\alpha(t)) - \omega_i t]} \quad (\text{S6})$$

where  $E_{l,\alpha}(\mathbf{q})$  is the amplitude of the scattered field.

The scattering vector  $\mathbf{q}$  is defined as  $\mathbf{q} = \mathbf{k}_i - \mathbf{k}_f$ , where  $\mathbf{k}_i$  and  $\mathbf{k}_f$  are the wave vectors of the incident and scattered waves, respectively. These wave vectors can be expressed as  $k_i = 2\pi n/\lambda_i$  and  $k_f = 2\pi n/\lambda_f$ , where  $\lambda_i$  and  $\lambda_f$  are the wavelengths of the incident and scattered waves and  $n$  is the refractive index of the medium. It is generally assumed that the wavelength does not undergo significant changes during scattering, so we can approximate  $|\mathbf{k}_i| \cong |\mathbf{k}_f|$ .

With this expression for  $\mathbf{q}$ , we can rewrite the equation for the field scattered by a particle (Eq. S6) as follows:

$$\mathbf{E}_{l,\alpha}(\mathbf{q}, t) = \mathbf{n}_i E_{l,\alpha}(\mathbf{q}) e^{i\mathbf{q} \cdot \mathbf{r}_\alpha(t)} e^{i(\mathbf{k}_f \cdot \mathbf{R} - \omega_i t)} \quad (\text{S7})$$

When calculating correlation functions, the phase term of the electric field is discarded because it does not depend on particle position. Therefore, it is convenient to work only with the amplitude of the electric field. Once the field scattered by a single colloidal particle is known, it is straightforward to find the field scattered by colloidal particles system.

Consider a volume  $V$  containing a large number of particles  $N$  in suspension that do not interfere with each other (that is, their positions are mutually independent). The total scattered electric field at a given  $\mathbf{q}$  will be the sum of the fields scattered by each individual particle at that  $\mathbf{q}$ . Therefore, the amplitude of the total field can be expressed as:

$$\mathbf{E}_l(\mathbf{q}, t) = \sum_{\alpha=1}^N E_{l,\alpha}(\mathbf{q}) e^{i\mathbf{q} \cdot \mathbf{r}_\alpha(t)} \quad (\text{S8})$$

As we can see, the fluctuations of the amplitude of the scattered electric field with time depend on the movement of each of the particles in suspension [1, 2].

In this section, we will focus on monodisperse systems, in which all particles are identical. Therefore, we can set  $E_{l,1}(q) = E_{l,2}(q) = \dots = E_l(q)$  and rewrite the Eq. (S8) as:

$$\mathbf{E}_l(\mathbf{q}, t) = \sum_{\alpha=1}^N E_l(\mathbf{q}) e^{i\mathbf{q} \cdot \mathbf{r}_\alpha(t)} \quad (\text{S9})$$

Our experiment enhances a standard DLS setup by introducing a design where two beams target the same sample, though at slightly different angles as shown in Fig. 1 of the main text. A detector measures the scattered intensity from these beams. Consequently, the electric field amplitude at the detector is formulated as [3–6]:

$$E(t) = E_1(\mathbf{q}_1, t) + E_2(\mathbf{q}_2, t) \quad (\text{S10})$$

Here,  $\mathbf{q}_l$  is each beam's scattering vector, and  $E_l(\mathbf{q}_l, t)$  denotes the scattered amplitude each beam directs to the detector for  $l = \{1, 2\}$ .

Using this expression for the scattered field, it is possible to define the electric field autocorrelation function in the case that there is a sum of electric fields  $G^{(1)}(\mathbf{q}_1, \mathbf{q}_2, \tau)$ . Inserting expression (S10) into (S4) we obtain:

$$\begin{aligned} G^{(1)}(\mathbf{q}_1, \mathbf{q}_2, \tau) &= \langle E(0)E^*(\tau) \rangle \\ &= \langle E_1(\mathbf{q}_1, 0)E_1^*(\mathbf{q}_1, \tau) \rangle + \langle E_1(\mathbf{q}_1, 0)E_2^*(\mathbf{q}_2, \tau) \rangle + \\ &\quad + \langle E_2(\mathbf{q}_2, 0)E_1^*(\mathbf{q}_1, \tau) \rangle + \langle E_2(\mathbf{q}_2, 0)E_2^*(\mathbf{q}_2, \tau) \rangle \end{aligned} \quad (\text{S11})$$

Using the definition of  $G^{(1)}(\mathbf{q}, \tau)$  given by Eq. (S4):

$$G^{(1)}(\mathbf{q}_1, \mathbf{q}_2, \tau) = G^{(1)}(\mathbf{q}_1, \tau) + \langle E_1(\mathbf{q}_1, 0)E_2^*(\mathbf{q}_2, \tau) \rangle + \langle E_2(\mathbf{q}_2, 0)E_1^*(\mathbf{q}_1, \tau) \rangle + G^{(1)}(\mathbf{q}_2, \tau) \quad (\text{S12})$$

In this expression, the terms where  $l = m$  refer to  $G^{(1)}(\mathbf{q}_1, \tau)$  and  $G^{(1)}(\mathbf{q}_2, \tau)$ . The cross terms where  $l \neq m$  equate to zero due to the absence of correlation between  $E_1(\mathbf{q}_1, t)$  and  $E_2(\mathbf{q}_2, t)$ .

To see this, the terms where  $l \neq m$  are expanded, following a similar derivation to cross-correlation derivations [3]. If we introduce the expression for the scattered electric field of each beam (S8) and by defining  $\Delta\mathbf{q} = \mathbf{q}_l - \mathbf{q}_m$  we arrive at the following expression:

$$\langle E_l(\mathbf{q}_l, 0)E_m^*(\mathbf{q}_m, \tau) \rangle = \sum_{\alpha, \beta=1}^N \left\langle E_{l, \alpha} E_{m, \beta} e^{i\mathbf{q}_l(\mathbf{r}_\alpha - \mathbf{r}'_\beta)} e^{-i\Delta\mathbf{q}\mathbf{r}'_\beta} \right\rangle \quad (\text{S13})$$

Particle coordinates with a prime refer to time  $\tau$ , while others are at time 0. It is assumed here that each beam illuminates an identical scattering volume.

For small values of  $\Delta\mathbf{q}$  the last exponential varies slowly. This allows us to separate the expected value of the product into the product of expected values. Moreover, since the system is monodisperse, the electric field amplitude solely depends on the magnitude of the scattering vector  $\mathbf{q}$  [2]. Given the small nature of  $\Delta\mathbf{q}$ , we can approximate  $E_{l, \alpha} = E_{m, \beta} = E_0$ :

$$\langle E_l(\mathbf{q}_l, 0)E_m^*(\mathbf{q}_m, \tau) \rangle = \sum_{\alpha, \beta=1}^N \left\langle E_0^2 e^{-i\Delta\mathbf{q}\mathbf{r}'_\beta} \right\rangle \left\langle e^{i\mathbf{q}_l(\mathbf{r}_\alpha - \mathbf{r}'_\beta)} \right\rangle \quad (\text{S14})$$

The last expected value matches the typical expression of  $g^{(1)}(\mathbf{q}_1, \tau)$  [1, 2]. This allows us to solve the spatial average, assuming our scattering volume is represented by a 3-D Gaussian with a  $1/e^2$ -radius  $R$  [3]:

$$\begin{aligned}\langle E_l(\mathbf{q}_l, 0)E_m^*(\mathbf{q}_m, \tau) \rangle &= n g^{(1)}(\mathbf{q}_l, \tau) \int d^3r E_l^2 e^{-2\mathbf{r}^2/R^2} e^{-i\Delta\mathbf{q}\cdot\mathbf{r}} \\ &= E_l^2 (\pi/2)^{3/2} n e^{-\Delta\mathbf{q}^2 R^2/8} g^{(1)}(\mathbf{q}_l, \tau)\end{aligned}\quad (\text{S15})$$

By comparing the relative weight of each term in expression (S12), we observe the following: In the case of  $l = m$  we get  $n E_l^2(q)(\pi/2)^{3/2} g^{(1)}(\mathbf{q}_l, \tau)$ . Conversely, for  $l \neq m$ , we see a difference factor of  $e^{-\Delta\mathbf{q}^2 R^2/8}$ .

This leads us to deduce that, for cross terms to vanish, the subsequent condition must be satisfied:

$$|\Delta\mathbf{q}|^{-1} < R \quad (\text{S16})$$

Knowing that our wavelength is  $\lambda = 632.8 \text{ nm}$  and  $\Delta\mathbf{q} = (2\pi n/\lambda)(0, 0, 2\sin(\phi))$  with refraction index  $n = 1.33$  and  $\phi = 0.052 \text{ rad}$ , we obtain  $|\Delta\mathbf{q}|^{-1} \approx 7 \cdot 10^{-7} \text{ m}$ , which is much lower than our beam radius  $R \in [10^{-5} \text{ m} - 10^{-4} \text{ m}]$ .

Given this context the electric field correlation function simplifies to:

$$g^{(1)}(\mathbf{q}_1, \mathbf{q}_2, \tau) \approx \frac{G^{(1)}(\mathbf{q}_1, \tau) + G^{(1)}(\mathbf{q}_2, \tau)}{G^{(1)}(\mathbf{q}_1, 0) + G^{(1)}(\mathbf{q}_2, 0)} = A_1 g^{(1)}(\mathbf{q}_1, \tau) + A_2 g^{(1)}(\mathbf{q}_2, \tau) \quad (\text{S17})$$

Where  $A_1$  and  $A_2$  are positive constants that take into account the relative field amplitude of each beam and possible misalignment of the scattering volumes and  $A_1 + A_2 = 1$ . The Siegert relation (S2) is altered by substituting Equation (S17), obtaining:

$$g^{(2)}(\mathbf{q}_1, \mathbf{q}_2, \tau) - 1 = \left| g^{(1)}(\mathbf{q}_1, \mathbf{q}_2, \tau) \right|^2 \quad (\text{S18})$$

With the acknowledgment that the function  $g^{(1)}(\mathbf{q}, \tau)$  with a drift velocity is determined by the expression  $g^{(1)}(\mathbf{q}, \tau) = e^{i\mathbf{q}\cdot\mathbf{v}\tau} e^{-Dq^2\tau}$  [2, 7–9]:

$$g^{(2)}(\mathbf{q}_1, \mathbf{q}_2, \tau) - 1 = \left| A_1 e^{i\mathbf{q}_1\cdot\mathbf{v}\tau} e^{-Dq_1^2\tau} + A_2 e^{i\mathbf{q}_2\cdot\mathbf{v}\tau} e^{-Dq_2^2\tau} \right|^2 \quad (\text{S19})$$

Since  $\Delta\mathbf{q}$  is very small,  $q_1 \approx q_2 \approx \bar{q} = |\mathbf{q}_1 + \mathbf{q}_2|/2$ , so last expression can be approximated to:

$$g^{(2)}(\mathbf{q}_1, \mathbf{q}_2, \tau) - 1 \approx \left| e^{-D\bar{q}^2\tau} (A_1 e^{i\mathbf{q}_1 \cdot \mathbf{v}\tau} + A_2 e^{i\mathbf{q}_2 \cdot \mathbf{v}\tau}) \right|^2 \quad (\text{S20})$$

and solving the square:

$$g^{(2)}(\mathbf{q}_1, \mathbf{q}_2, \tau) - 1 = e^{-2D\bar{q}^2\tau} (A_1^2 + A_2^2 + 2A_1A_2 \cos(\Delta\mathbf{q} \cdot \mathbf{v}\tau)) \quad (\text{S21})$$

In an experimental case in which the intensities of both beams are not the same, the previous expression turns to:

$$g^{(2)}(\mathbf{q}_1, \mathbf{q}_2, \tau) - 1 = e^{-2D\bar{q}^2\tau} [(1 - C) + C \cos(\Delta\mathbf{q} \cdot \mathbf{v}\tau)] \quad (\text{S22})$$

where  $C \in [0 - 0.5]$  is a constant.

Lastly we want to take into account the effect of particles leaving the scattering volume. For doing so, it is defined a position dependent field amplitude. Since in our experiment the velocity is completely vertical, it is assumed that particles only exit the volume through the  $z$  direction. The position dependent field amplitude is:

$$P(z) = \begin{cases} \frac{1}{h} & \text{if } -h/2 \leq z \leq h/2 \\ 0 & \text{otherwise} \end{cases} \quad (\text{S23})$$

Where  $h$  is the beam thickness. We go back to equation (S14), using  $l = m$  so  $\Delta\mathbf{q} = 0$  and taking into account that different particles do not interact:

$$G^{(1)}(\mathbf{q}, \tau) = \langle E(\mathbf{q}, 0) E^*(\mathbf{q}, \tau) \rangle = \sum_{\alpha=1}^N \langle E_0^2 P(z_\alpha(0)) P(z_\alpha(\tau)) \rangle \langle e^{i\mathbf{q}(\mathbf{r}_\alpha - \mathbf{r}'_\alpha)} \rangle \quad (\text{S24})$$

where  $z_\alpha(t) = z_0 + vt$  is the  $z$ -coordinate of the particle  $\alpha$ . Assuming that the particles are equally distributed, the first average is straightforward and the normalized correlation function is:

$$g^{(1)}(\mathbf{q}, \tau) = \left(1 - \frac{v\tau}{h}\right) \langle e^{i\mathbf{q}(\mathbf{r}_\alpha - \mathbf{r}'_\alpha)} \rangle = \left(1 - \frac{v\tau}{h}\right) e^{i\mathbf{q} \cdot \mathbf{v}\tau} e^{-Dq^2\tau} \quad (\text{S25})$$

with  $\tau \leq h/v$  and using this expression into Eqs. (S17, S18):

$$g^{(2)}(\mathbf{q}_1, \mathbf{q}_2, \tau) - 1 = e^{-2D\bar{q}^2\tau} [(1 - C) + C \cos(\Delta\mathbf{q} \cdot \mathbf{v}\tau)] \left(1 - \frac{v\tau}{h}\right)^2 \quad (\text{S26})$$

## B. Two-Velocity One-Laser Single-Detector Correlation Function in Dynamic Light Scattering

We now consider a new configuration with respect to the one described in section A: a single laser, a single detector and two distinct velocities. In this configuration, we employ a single scattering vector  $\mathbf{q}$  but allow for two distinct drift velocities  $\mathbf{v}_1$  and  $\mathbf{v}_2$ . This scenario is relevant when the colloidal system contains two populations of particles moving at different velocities, either due to different driving forces or differing interactions with the medium.

The intensity autocorrelation function  $g^{(2)}(\mathbf{q}, \tau)$  is given by the same fundamental definition:

$$g^{(2)}(\mathbf{q}, \tau) = \frac{\langle I(\mathbf{q}, 0)I(\mathbf{q}, \tau) \rangle}{\langle I(\mathbf{q}, 0) \rangle^2} \quad (\text{S27})$$

Using the Siegert relation, we connect  $g^{(2)}(\mathbf{q}, \tau)$  with the electric field correlation function  $g^{(1)}(\mathbf{q}, \tau)$ :

$$g^{(2)}(\mathbf{q}, \tau) = 1 + |g^{(1)}(\mathbf{q}, \tau)|^2 \quad (\text{S28})$$

Given the two distinct drift velocities, the total scattered electric field at the detector can be expressed as the sum of the fields corresponding to each velocity:

$$E(t) = E_1(\mathbf{q}, t) + E_2(\mathbf{q}, t) \quad (\text{S29})$$

Inserting this into the definition of the electric field correlation function  $G^{(1)}(\mathbf{q}, \tau)$  (Eq. S4) and assuming there is no correlation between  $E_1$  and  $E_2$ , the cross terms  $\langle E_1(\mathbf{q}, 0)E_2^*(\mathbf{q}, \tau) \rangle$  and  $\langle E_2(\mathbf{q}, 0)E_1^*(\mathbf{q}, \tau) \rangle$  vanish. Thus, the correlation function simplifies to:

$$G^{(1)}(\mathbf{q}, \tau) = G_1^{(1)}(\mathbf{q}, \tau) + G_2^{(1)}(\mathbf{q}, \tau) \quad (\text{S30})$$

Utilizing the normalized electric field correlation function  $g^{(1)}(\mathbf{q}, \tau) = \frac{G^{(1)}(\mathbf{q}, \tau)}{G^{(1)}(\mathbf{q}, 0)}$ , we can express:

$$g^{(1)}(\mathbf{q}, \tau) = B_1 g_1^{(1)}(\mathbf{q}, \tau) + B_2 g_2^{(1)}(\mathbf{q}, \tau) \quad (\text{S31})$$

Here,  $B_1$  and  $B_2$  are the weighting factors corresponding to the proportion of particles with each velocity component, satisfying  $B_1 + B_2 = 1$ .

The electric field correlation function for particles with drift velocity is given by  $g^{(1)}(\mathbf{q}, \tau) = e^{i\mathbf{q} \cdot \mathbf{v}\tau} e^{-Dq^2\tau}$  [2, 7–9]. For the system with two velocities, this becomes:

$$g_1^{(1)}(\mathbf{q}, \tau) = e^{i\mathbf{q} \cdot \mathbf{v}_1 \tau} e^{-D_1 q^2 \tau}, \quad g_2^{(1)}(\mathbf{q}, \tau) = e^{i\mathbf{q} \cdot \mathbf{v}_2 \tau} e^{-D_2 q^2 \tau} \quad (\text{S32})$$

Substituting these into Equation (S31), we get:

$$g^{(1)}(\mathbf{q}, \tau) = B_1 e^{i\mathbf{q} \cdot \mathbf{v}_1 \tau} e^{-D_1 q^2 \tau} + B_2 e^{i\mathbf{q} \cdot \mathbf{v}_2 \tau} e^{-D_2 q^2 \tau} \quad (\text{S33})$$

Using the Siegert relation (S28), we obtain:

$$g^{(2)}(\mathbf{q}, \tau) - 1 = \left| B_1 e^{i\mathbf{q} \cdot \mathbf{v}_1 \tau} e^{-D_1 q^2 \tau} + B_2 e^{i\mathbf{q} \cdot \mathbf{v}_2 \tau} e^{-D_2 q^2 \tau} \right|^2 \quad (\text{S34})$$

Simplifying further, we have:

$$g^{(2)}(\mathbf{q}, \tau) - 1 = B_1^2 e^{-2D_1 q^2 \tau} + B_2^2 e^{-2D_2 q^2 \tau} + 2B_1 B_2 \cos(\mathbf{q} \cdot \Delta \mathbf{v} \tau) e^{-(D_1 + D_2) q^2 \tau} \quad (\text{S35})$$

where  $\Delta \mathbf{v} = \mathbf{v}_1 - \mathbf{v}_2$ .

This final expression provides the intensity autocorrelation function for a system with one scattering vector and two distinct drift velocities, extending the model developed in the previous section. It is important to notice that for obtaining oscillations, the dot product must not be 0, so in the case of a vertical velocities the scattering vector must not be in the scattering plane.

### C. Technical Details of Fluid Dynamics Simulations

Using the Nonisothermal Flow interface in COMSOL, free convection was modeled in water, taking into account both momentum and energy balances. The simulations aimed to provide insights into heat transfer through convection and conduction within the setup. The initial conditions were set as  $T_{\text{Room}} = 23^\circ\text{C}$  for both the cell and water. The cylindrical glass cell's base was positioned in a thermostatised bath that heated only its bottom-most 1 cm. This section of the external surface of the cell maintained a constant temperature, mirroring the bath's temperature. The remaining cell's side walls, which were not submerged in the bath, were in direct contact with a metal component maintained at room temperature, leading to a constant lateral temperature boundary for the cell. Internally, the boundary between the water and glass adhered to a no-slip condition, while the open surface of the water, subject to ambient conditions, was characterized by a slip condition.

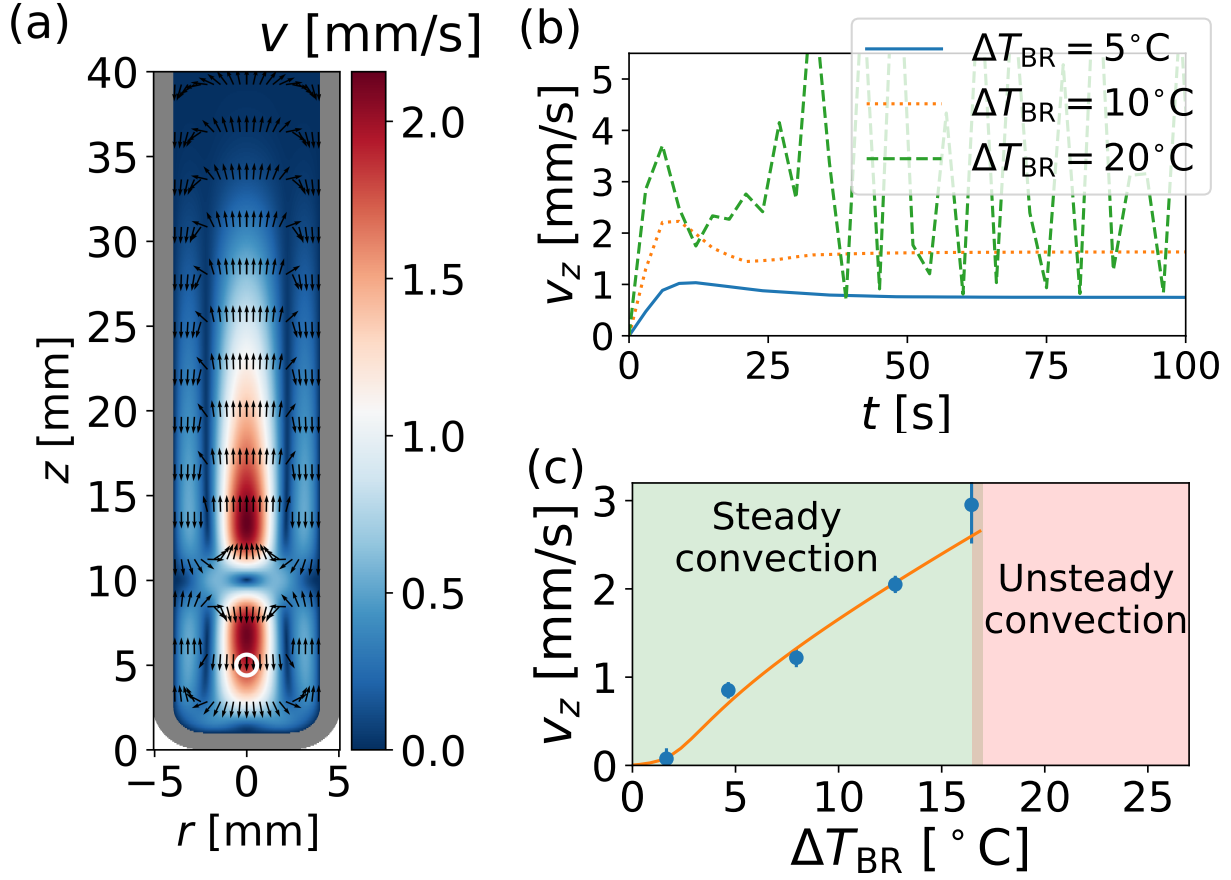

FIG. S2. Predictions obtained by COMSOL simulations. (a) Velocity profile in stationary conditions, for a temperature gradient given by  $\Delta T_{BR} = 10^\circ\text{C}$ . The white circle denotes the measurement point in our DLS device. (b) Time evolution of  $v_z$  at the measurement point for different temperature gradients. (c)  $v_z$  at the measurement point as a function of the temperature difference,  $\Delta T_{BR}$  (line). Symbols represent the experimental data, obtained from the average over ten independent DLS measurements using Eq. (S26).

This model was used to explore the system response over time to a temperature difference between the bath and the room of  $\Delta T_{BR} = 10^\circ\text{C}$ , at which oscillatory behavior in the correlation function was observed in our experiments. For this condition, the fluid dynamics simulation revealed that both the velocity and temperature profiles within the cell eventually reach a steady state. The stationary velocity profile is depicted in Fig. S2(a), with the experimental measurement point highlighted by a circle, inside which magnitudes vary less than 1%, and the drift velocities are completely vertical. The temperature there is lower than the bath temperature as an effect of the convection currents. We observe two convective regions above and below the bath level.

However, when  $\Delta T_{BR}$  becomes significantly large, the system dynamics undergo significant al-

terations. This is evident from Figure S2(b), where the time evolution of vertical velocity at the measuring point for different  $\Delta T_{\text{BR}}$  is presented. For  $\Delta T_{\text{BR}}$  of 5°C and 10°C, the system stabilizes between 30 to 40 s. However, at  $\Delta T_{\text{BR}} = 20^\circ\text{C}$ , a steady state is unattainable, indicating a transition to a non-stationary regime. This behavior aligns entirely with the experimental observations, which identifies two regimes based on the  $\Delta T_{\text{BR}}$ .

A physical description of the stationary to non-stationary transition observed in both experiments and fluid dynamics simulations can be explained in terms of the Rayleigh number ( $\text{Ra} = \frac{g\beta\Delta TL^3}{\nu\alpha}$ ), which compares the time scales for thermal transport via diffusion and via convection. According to the literature, there is a critical value,  $\text{Ra}_c$ , at which the fluid transits from a laminar steady convection state towards a laminar but unsteady convection regime that depends on the geometry [10–13]. Using the experimental values of the height of the measurement cell ( $L = 3.0$  cm), thermal diffusivity of water ( $\alpha = 1.43 \cdot 10^{-7} \text{ m}^2/\text{s}$ ), kinematic viscosity ( $\nu = 8 \cdot 10^{-7} \text{ m}^2/\text{s}$ ), gravity ( $g = 9.81 \text{ m/s}^2$ ), thermal expansion coefficient ( $\beta = 4 \cdot 10^{-4} \text{ K}^{-1}$ ), and temperature difference at the transition, we find that  $\text{Ra}_c \approx 1.5 \cdot 10^7$ , which agrees with the value reported in the literature for a similar cell geometry using adiabatic walls [14].

- 
- [1] B. J. Berne and R. Pecora, *Dynamic light scattering: with applications to chemistry, biology, and physics* (Courier Corporation, 2000).
  - [2] R. Pecora, *Dynamic light scattering: applications of photon correlation spectroscopy* (Springer Science & Business Media, 1985).
  - [3] K. Schätzel, *Journal of modern optics* **38**, 1849 (1991).
  - [4] L. B. Aberle, P. Hülstede, S. Wiegand, W. Schröer, and W. Staude, *Applied Optics* **37**, 6511 (1998).
  - [5] G. D. Phillies, *The Journal of Chemical Physics* **74**, 260 (1981).
  - [6] P. Pusey, *Current opinion in colloid & interface science* **4**, 177 (1999).
  - [7] E. Moulin, I. A. Nyrkova, N. Giuseppone, A. N. Semenov, and E. Buhler, *Soft Matter* **16**, 2971 (2020).
  - [8] A. Sehgal and T. A. Seery, *Macromolecules* **32**, 7807 (1999).
  - [9] K. Katayama, H. Nomura, H. Ogata, and T. Eitoku, *Physical Chemistry Chemical Physics* **11**, 10494 (2009).
  - [10] S. Chandrasekhar, *Hydrodynamic and hydromagnetic stability* (Courier Corporation, 2013).
  - [11] R. Clever and F. Busse, *Journal of Fluid Mechanics* **65**, 625 (1974).

- [12] J. Patterson and J. Imberger, *Journal of Fluid Mechanics* **100**, 65 (1980).
- [13] P. Oresta, G. Stringano, and R. Verzicco, *European Journal of Mechanics-B/Fluids* **26**, 1 (2007).
- [14] P. Le Quéré, *Physics of Fluids A: Fluid Dynamics* **2**, 503 (1990).
